# Supplementary material for: Amplification of the diamagnetic response in small Hubbard rings
Source: arXiv:1607.07473 ancillary file (2016-07-25)
Supplement: Supplementary file 1 [file Supplementary_material_Trevisan_Caldeira.pdf]

# Supplementary Material

**Article title:** Amplification of the diamagnetic response in small Hubbard rings

**Author(s):** T. V. Trevisan and A. O. Caldeira

The goal of this Supplementary Material is to provide the reader with more details about (i) the energy spectrum of the rings and how this spectrum changes when we add our extra interaction term ($\hat{H}_I$) to the Hubbard Hamiltonian (evidencing the level crossings between the ground state and some excited state of the system), as well as (ii) the behavior of the persistent current that is established in the ground state of the rings as functions of both the magnetic flux $f$ that pierces the ring and the on-site repulsion, and (iii) the maps of the parameter space $\Delta_1 \times U$. We also provide a demonstration of the expressions of the current operator for the Hubbard model and our extension thereof.

## I. INFLUENCE OF $\hat{\mathrm{H}}_{\mathrm{I}}$ ON THE ENERGY SPECTRUM OF THE RINGS

The figures on the left half of the page show the energy spectrum of the Hubbard Hamiltonian for rings with (a) three sites and two electrons, (c) three sites and three electrons, (e) four sites and three electrons, (h) five sites and five electrons, (j) six sites and two electrons, and (l) six sites and six electrons. The figures on the right half of the page refer to the same systems as those of the figures on the left, respectively, but now the energy spectrum is obtained through our extension of the Hubbard model (*i.e.* $\Delta_1 \neq 0$ and/or $\Delta_2 \neq 0$). In each one of the figures on the right, we show the value of the on-site repulsion $U_0$ at which the level crossing between the ground state and some excited state of the rings takes place. Besides, in Figs. 1(i), (k) and (m) we show only the ground state level and the next four excited states in order to ease the visualization of the level crossings.

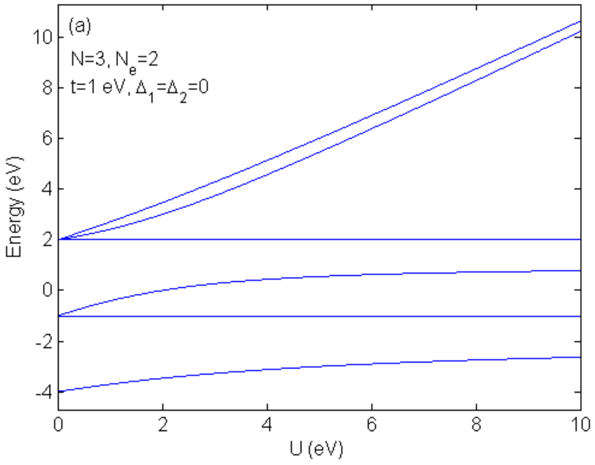


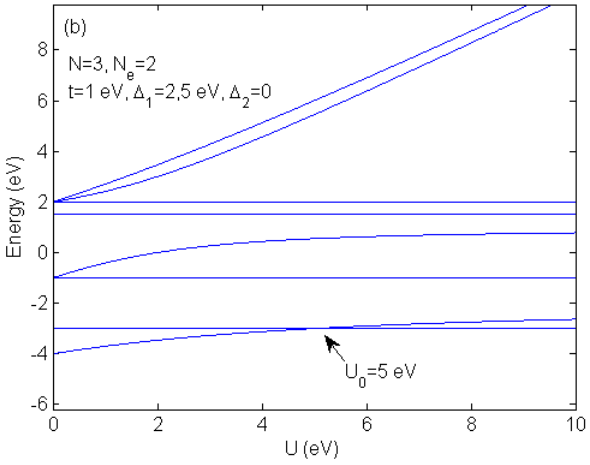

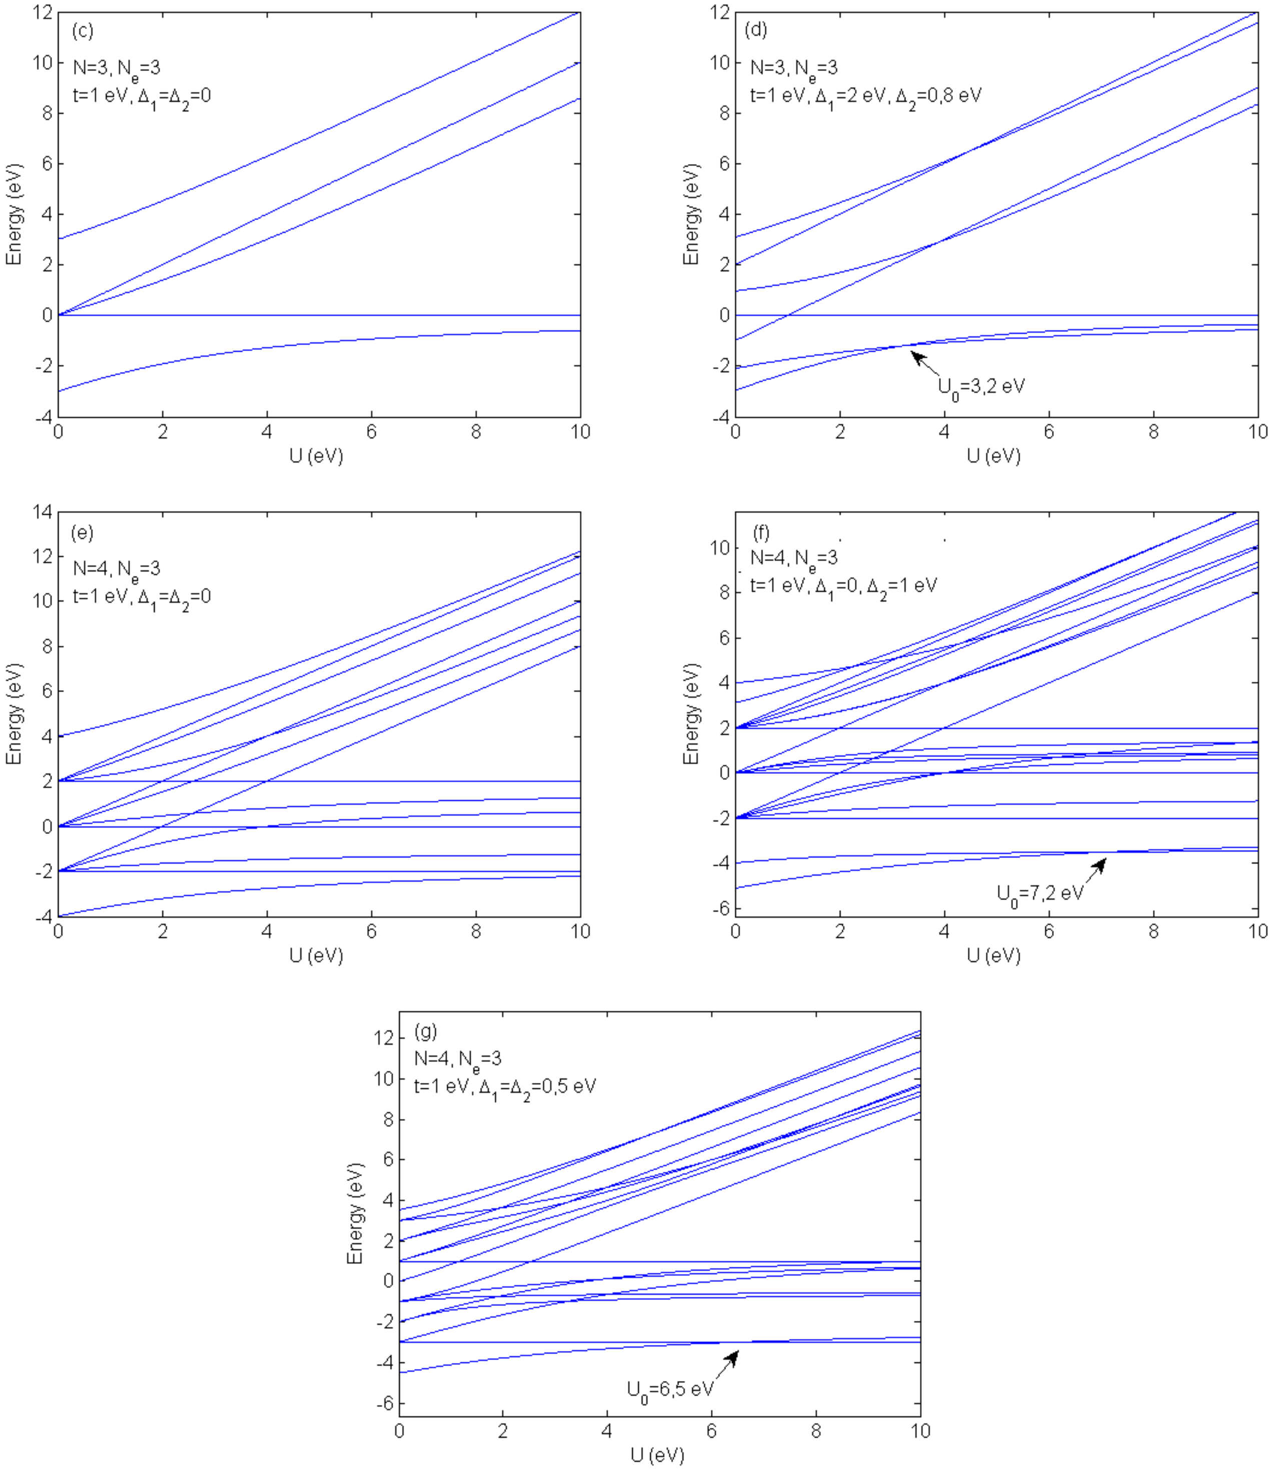

(c)
N=3, $N_e$=3
t=1 eV, $\Delta_1$=$\Delta_2$=0
Energy (eV)
U (eV)
(d)
N=3, $N_e$=3
t=1 eV, $\Delta_1$=2 eV, $\Delta_2$=0,8 eV
$U_0$=3,2 eV
Energy (eV)
U (eV)
(e)
N=4, $N_e$=3
t=1 eV, $\Delta_1$=$\Delta_2$=0
Energy (eV)
U (eV)
(f)
N=4, $N_e$=3
t=1 eV, $\Delta_1$=0, $\Delta_2$=1 eV
$U_0$=7,2 eV
Energy (eV)
U (eV)
(g)
N=4, $N_e$=3
t=1 eV, $\Delta_1$=$\Delta_2$=0,5 eV
$U_0$=6,5 eV
Energy (eV)
U (eV)

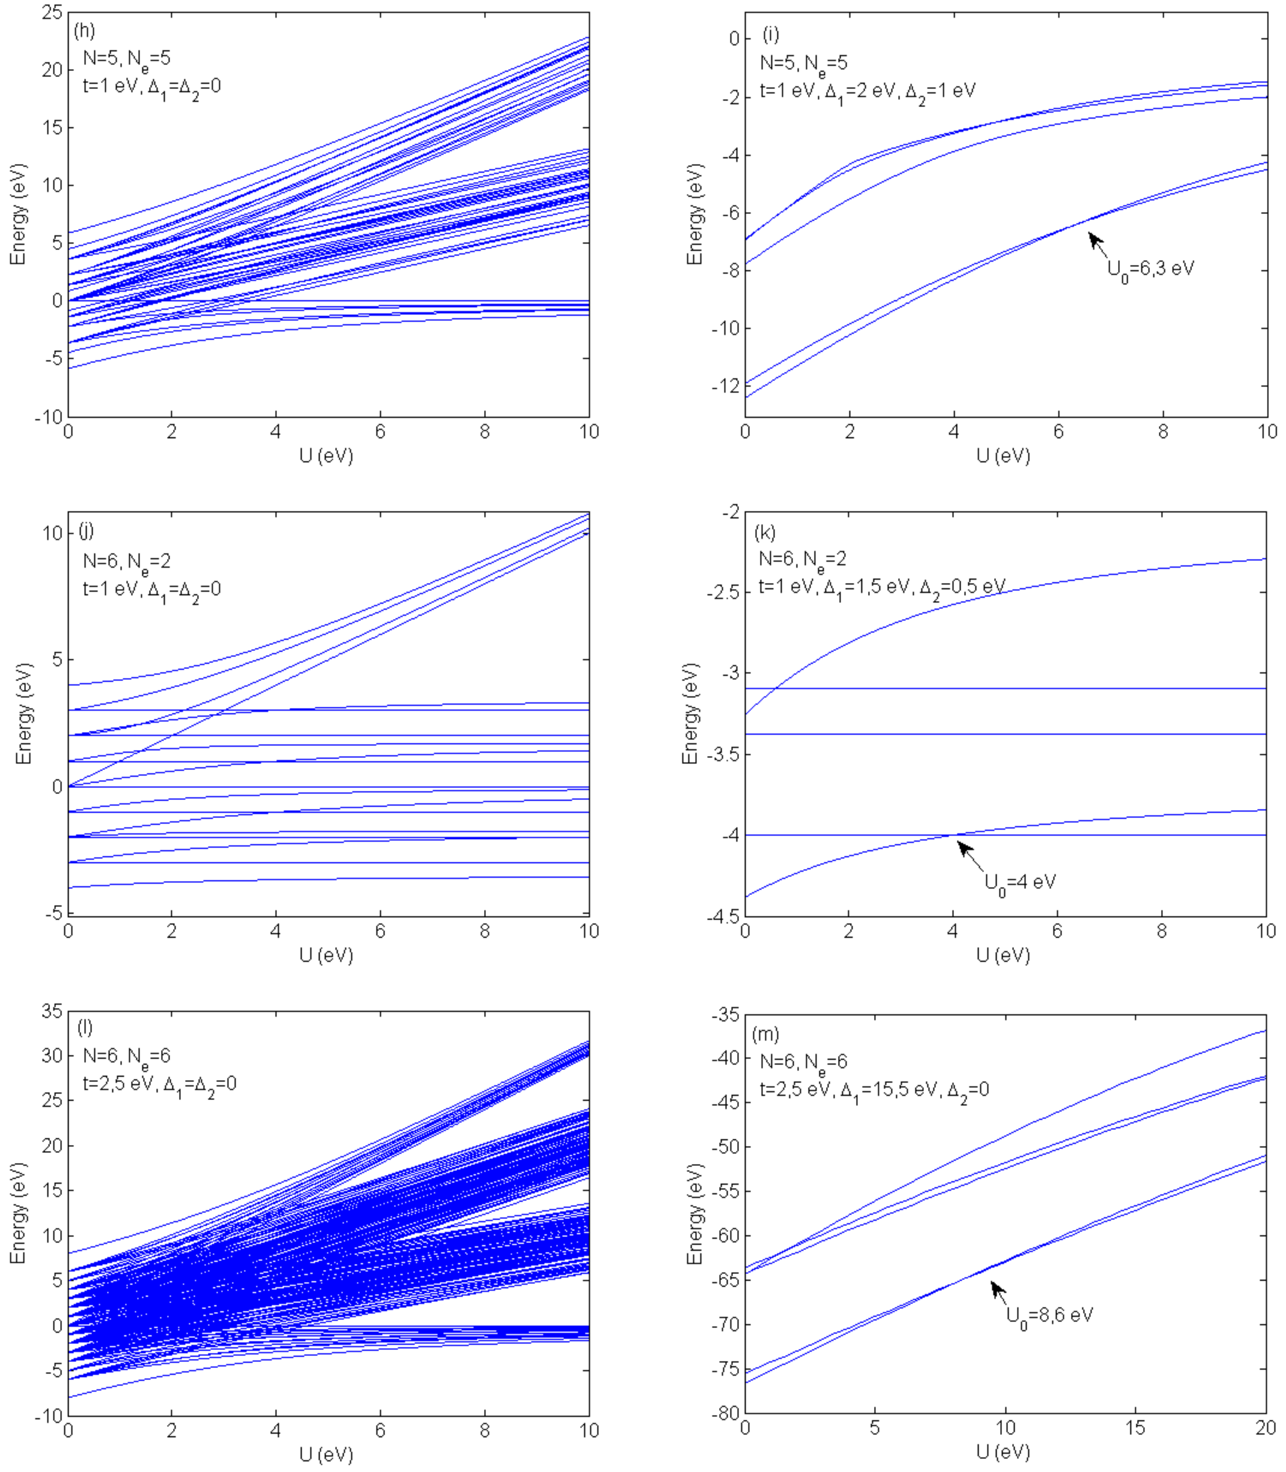


FIG. 1. Energy levels, as a function of the on-site repulsion, of rings with $N = 3$ sites and $N_e = 2$ electrons ((a) and (b)), $N = 3$ sites and $N_e = 3$ electrons ((c) and (d)), $N = 4$ sites and $N_e = 3$ electrons ((e), (f) and (g)), $N = 5$ sites and $N_e = 5$ electrons ((h) and (i)), $N = 6$ sites and $N_e = 2$ electrons ((j) and (k)) and $N = 6$ sites and $N_e = 6$ electrons ((l) and (m)). The energy levels shown in the figures (b), (d), (f), (g), (i), (k) and (m) were calculated through our extension of the Hubbard model ($\Delta_{\sigma\sigma'} \neq 0$), while the others refer to the Hubbard Hamiltonian without the extra interaction term. The values of $\Delta_1$ and $\Delta_2$ chosen in each case, as well as the on-site repulsion $U_0$ at which the level crossing occur are indicated in each figure. We set the hopping parameter $t = 1\,eV$, except for figures (l) and (m), where we used $t = 2,5\,eV$.

## II. CURRENT OPERATOR

In this section, we deduce the expressions of the current operator for the Hubbard model and our extension thereof. The obtainment of the current operator for the Hubbard model can be easily found in the literature[1]. However, we will repeat it here in order to comment upon a detail that is usually neglected in many references.

### A. Current Operator for the Hubbard model

We start with the continuity equation,

$$e\frac{\partial \hat{n}_{m\sigma}}{\partial t} + \hat{\jmath}_{m\sigma} - \hat{\jmath}_{(m-1)\sigma} = 0\,, \tag{1}$$

which holds for each of the $m = 1, 2, 3, \cdots, N$ sites of the ring, since we have a stationary current flowing in the system. In Eq. (1), $e < 0$ is the electronic charge. According to the Heisenberg picture, the time derivative of the number operator $\hat{n}_{m\sigma} = c^{\dagger}_{m\sigma}c_{m\sigma}$ is related to its commutator with the Hamiltonian of the system,

$$\frac{\partial \hat{n}_{m\sigma}}{\partial t} = i\left[\hat{H}, \hat{n}_{m\sigma}\right]\,, \tag{2}$$

where $\hat{H}$ is, in this case, the Hubbard Hamiltonian,

$$\hat{H} = -t\sum_{i=1}^{N}\sum_{\sigma=\uparrow,\downarrow}\left(c^{\dagger}_{i\sigma}c_{(i+1)\sigma} + h.c.\right) + U\sum_{i=1}^{N}\hat{n}_{i\uparrow}\hat{n}_{i\downarrow}\,. \tag{3}$$

Using the anticommutation relations of the fermion creation and annihilation operators,

$$\begin{array}{c}\left\{c_{m\sigma}, c^{\dagger}_{i\sigma'}\right\} = \delta_{m,i}\delta_{\sigma,\sigma'}\\ \left\{c_{m\sigma}, c_{i\sigma'}\right\} = \left\{c^{\dagger}_{m\sigma}, c^{\dagger}_{i\sigma'}\right\} = 0\end{array}\,, \tag{4}$$

as well as the properties $[AB, C] = A[B, C] + [A, C]B$ and $[A, BC] = \{A, B\}C - B\{A, C\}$, we find

$$\sum_{i=1}^{N}\left[\hat{n}_{i\uparrow}\hat{n}_{i\downarrow}, \hat{n}_{m\sigma}\right] = 0$$

and, hence,

$$\begin{aligned}\left[\hat{H}, \hat{n}_{m\sigma}\right] &= -t\sum_{i=1}^{N}\sum_{\sigma'}\left\{\left[c^{\dagger}_{i\sigma'}c_{(i+1)\sigma'}, \hat{n}_{m\sigma}\right] + \left[c^{\dagger}_{(i+1)\sigma'}c_{i\sigma'}, \hat{n}_{m\sigma}\right]\right\}\\ &= t\left(c^{\dagger}_{m\sigma}c_{(m+1)\sigma} - c^{\dagger}_{(m+1)\sigma}c_{m\sigma} - c^{\dagger}_{(m-1)\sigma}c_{m\sigma} + c^{\dagger}_{m\sigma}c_{(m-1)\sigma}\right)\end{aligned}\,. \tag{5}$$

Substituting Eq.(5) into Eq.(2), we obtain

$$\frac{\partial \hat{n}_{m\sigma}}{\partial t} = it\left(c^{\dagger}_{m\sigma}c_{(m+1)\sigma} - c^{\dagger}_{(m+1)\sigma}c_{m\sigma} - c^{\dagger}_{(m-1)\sigma}c_{m\sigma} + c^{\dagger}_{m\sigma}c_{(m-1)\sigma}\right) \tag{6}$$

and comparing Eq.(6) with Eq.(1) we can identify

$$\hat{j}_{m\sigma} = -iet\left(c^{\dagger}_{m\sigma}c_{(m+1)\sigma} - h.c.\right) \ , \tag{7}$$

as well as

$$\hat{j}_{(m-1)\sigma} = -iet\left(c^{\dagger}_{(m-1)\sigma}c_{m\sigma} - h.c.\right) \ . \tag{8}$$

The total current operator, $\hat{\mathscr{I}}_{el}$, is given by the summation of $\hat{j}_{m\sigma}$ over all sites of the ring and over the spin $\sigma =\uparrow,\downarrow$ of the electrons, yielding

$$\hat{\mathscr{I}}_{el} = -\frac{iet}{N}\sum_{m=1}^{N}\sum_{\sigma}\left(c^{\dagger}_{m\sigma}c_{(m+1)\sigma} - c^{\dagger}_{(m+1)\sigma}c_{m\sigma}\right) \ . \tag{9}$$

It is important to note that we must add the factor $1/N$ before the summation over the sites of the rings, since the current that passes through the $m$-th site of the ring is the same that passes through the other sites, otherwise, we would have a non realistic amplification of the local value of the charge flux. In other words, without the factor $1/N$, we would count the same electric current $N$ times. Some references[1] neglect this fact and present an expression for the current operator without the $1/N$ factor, while in other references[2], we find an expression for the current operator consistent with Eq.(9).

In the presence of an external magnetic field $\vec{B} = B\hat{z}$, because of the minimal coupling $\vec{P} \to \vec{P} - e\vec{A}/c$ (where $\vec{A}$ is the vector potential related to the magnetic field, $\vec{B} = \vec{\nabla}\times\vec{A}$), the Wannier wave functions acquire a phase factor (Gauge transformation)[1] $\tilde{\phi}(\vec{r}-\vec{R}_j) = e^{i|e|\lambda(\vec{R}_j)/c}\phi(\vec{r}-\vec{R}_j)$, and consequently, the fermion operators are also modified:

$$\tilde{c}^{\dagger}_{j\sigma} = e^{-i|e|\lambda(\vec{R}_j)/c}c^{\dagger}_{j\sigma} \ , \tag{10}$$

with

$$\lambda(\vec{R}_j) = \int_{\vec{r}_0}^{\vec{R}_j}\vec{A}(\vec{r})\cdot d\vec{r} \ , \tag{11}$$

where $\vec{R}_j$ is the vector position of the $j$-th site of the ring and $\vec{r}_0$ is an arbitrary reference position. Substituting Eq.(10) into

Eq.(9), we find the expression for the total current operator for the Hubbard model in the presence of the field $\vec{B} = B\hat{z}$,

$$\hat{\mathscr{J}}_{mag} = -\frac{iet}{N}\sum_{j=1}^{N}\sum_{\sigma}\left(e^{i2\pi f/N}c^{\dagger}_{j\sigma}c_{(j+1)\sigma} - e^{-i2\pi f/N}c^{\dagger}_{(j+1)\sigma}c_{j\sigma}\right) \,, \tag{12}$$

where we used $|e|[\lambda(\vec{R}_{j+1}) - \lambda(\vec{R}_j)]/c = 2\pi f/N$, with $f \equiv \phi/\phi_0$ the dimensionless magnetic flux that pierces the ring and $\phi_0 = hc/|e|$, the flux quantum.

Alternatively, Eq.(12) could have been found had we evaluated the commutator of Eq.(2) with $\hat{H}$ given by

$$\hat{H} = -t\sum_{j=1}^{N}\sum_{\sigma}\left(e^{i2\pi f/N}c^{\dagger}_{j\sigma}c_{(j+1)\sigma} + h.c.\right) + U\sum_{j=1}^{N}\hat{n}_{j\uparrow}\hat{n}_{j\downarrow} - \mu_B B\sum_{j=1}^{N}(\hat{n}_{j\uparrow} - \hat{n}_{j\downarrow}) \,, \tag{13}$$

instead of Eq.(3).

### B. Current Operator for the extension of the Hubbard model

In this case, the total Hamiltonian of the system is given by

$$\hat{H} = -t\sum_{j=1}^{N}\sum_{\sigma=\uparrow,\downarrow}\left(c^{\dagger}_{j\sigma}c_{(j+1)\sigma} + h.c.\right) + U\sum_{j=1}^{N}\hat{n}_{j\uparrow}\hat{n}_{j\downarrow} + \hat{H}_I \,, \tag{14}$$

where

$$\hat{H}_I = -\sum_{\sigma,\sigma'}\Delta_{\sigma\sigma'}\sum_{j=1}^{N}\left(c^{\dagger}_{j\sigma}c^{\dagger}_{(j-1)\sigma'}c_{(j-2)\sigma'}c_{(j-1)\sigma} + h.c.\right) \,, \tag{15}$$

with $\Delta_{\sigma\sigma'}$ being an adjustable energy-dimension positive parameter

$$\Delta_{\sigma\sigma'} = \begin{cases} \Delta_1 \,, & \text{if } \sigma = \sigma' \\ \Delta_2 \,, & \text{if } \sigma \neq \sigma' \end{cases} \,. \tag{16}$$

Since the commutator $[\hat{H}_I, \hat{n}_{m\sigma}]$ is not zero, it follows that Eq.(9) is not the adequate expression for the current operator for our extension of the Hubbard model.

In order to find the new expression for the current operator, we repeat the procedure of subsection II A, and evaluate $[\hat{H}, \hat{n}_{m\sigma}]$, with $\hat{H}$ given by Eq.(14). We find, in this case,

$$\begin{aligned}\hat{j}_{m\sigma} = -it\left(c^{\dagger}_{m\sigma}c_{(m+a)\sigma} - h.c.\right) + i\sum_{\sigma'}\Delta_{\sigma'\sigma}\Big[\Big(&c^{\dagger}_{(m+1)\sigma}c^{\dagger}_{m\sigma'}c_{(m-1)\sigma'}c_{m\sigma} + \\ &+ c^{\dagger}_{(m+2)\sigma'}c^{\dagger}_{(m+1)\sigma}c_{m\sigma}c_{(m+1)\sigma'}\Big) - h.c.\Big] \,.\end{aligned} \tag{17}$$

Hence, summing over the sites of the ring and the electronic spin degrees of freedom, we have

$$\hat{\mathscr{I}}_{el}^{(II)} = -\frac{iet}{N}\sum_{j=1}^{N}\sum_{\sigma}\left(c_{j\sigma}^{\dagger}c_{(j+1)\sigma} - h.c.\right) + \frac{2ie}{N}\sum_{\sigma,\sigma'}\sum_{j=1}^{N}\left(c_{j\sigma}^{\dagger}c_{(j-1)\sigma'}^{\dagger}c_{(j-2)\sigma'}c_{(j-1)\sigma} - h.c.\right) \ , \tag{18}$$

where the index "$(II)$" is used to differ Eq.(18) from Eq.(9). Note, again the factor $1/N$ to avoid counting several times the same current.

Now, in the presence of an external magnetic field $\vec{B} = B\hat{z}$, substituting Eq.(10) into Eq.(18), we have

$$\begin{array}{c} \hat{\mathscr{I}}_{mag}^{(II)} = -\frac{iet}{N}\sum_{j=1}^{N}\sum_{\sigma}\left(e^{i2\pi f/N}c_{j\sigma}^{\dagger}c_{(j+1)\sigma} - h.c.\right) + \\ +\frac{2ie}{N}\sum_{\sigma,\sigma'}\sum_{j=1}^{N}\left(e^{-i4\pi f/N}c_{j\sigma}^{\dagger}c_{(j-1)\sigma'}^{\dagger}c_{(j-2)\sigma'}c_{(j-1)\sigma} - h.c.\right) \end{array} . \tag{19}$$

## III. MAPS OF THE PARAMETER SPACE $\Delta_1 \times U$

The figures of this section are color maps of the parameter space $\Delta_1 \times U$ in the absence of an external magnetic field and for $t$ and $\Delta_2$ fixed. They indicate whether the ground state of the rings with (a) three and (b) five sites at half-filling, as well as (c) and (d) four sites and three electrons can be a current-carrying state according to our extension of the Hubbard model: the green regions represent points $(\Delta_1, U)$ for which the matrix representation of the current operator, Eq.(18), in the subspace of the ground state is non-zero. Thus, in this case, there is at least one linear combination of the $g_0$ degenerated ground states of the ring for which the expected value of the current operator is different from zero, meaning that the ground state can be a current-carrying state. On the other hand, the red regions are points $(\Delta_1, U)$ such as the matrix representation of the current operator is identically zero, and consequently, for these vales of the parameters $\Delta_1$ and $U$, the ground state cannot be a current-carrying state, independently of the linear combination we choose. Besides, Figs. 2(e) and (f) are maps for rings with an even number $N_e$ of electrons (independently of the number of sites of the system), with $N_e$ a multiple of four and, necessarily $\Delta_2 = 0$, in the case of Fig. 2(f)

Note that, according to the map in Fig. 2(f), the ground state of rings with an even number of electrons can be a current-carrying state only if $N_e$ is a multiple of four and $U = \Delta_1 = \Delta_2 = 0$. This is so because the ground state of the non-interacting problem ($U = \Delta_1 = \Delta_2 = 0$) with an even number of electrons is degenerated (and the matrix representation of the current operator in the subspace of the ground state in non-zero) only when $N_e$ is a multiple of four. When we turn on the interactions between the electrons, we break this degeneracy.

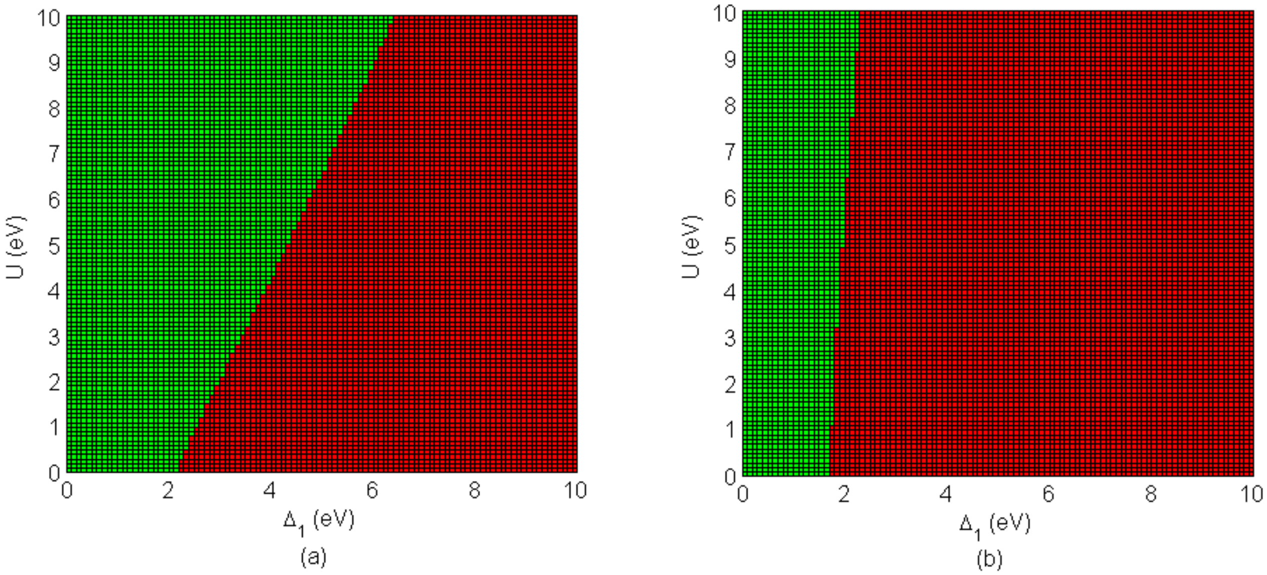

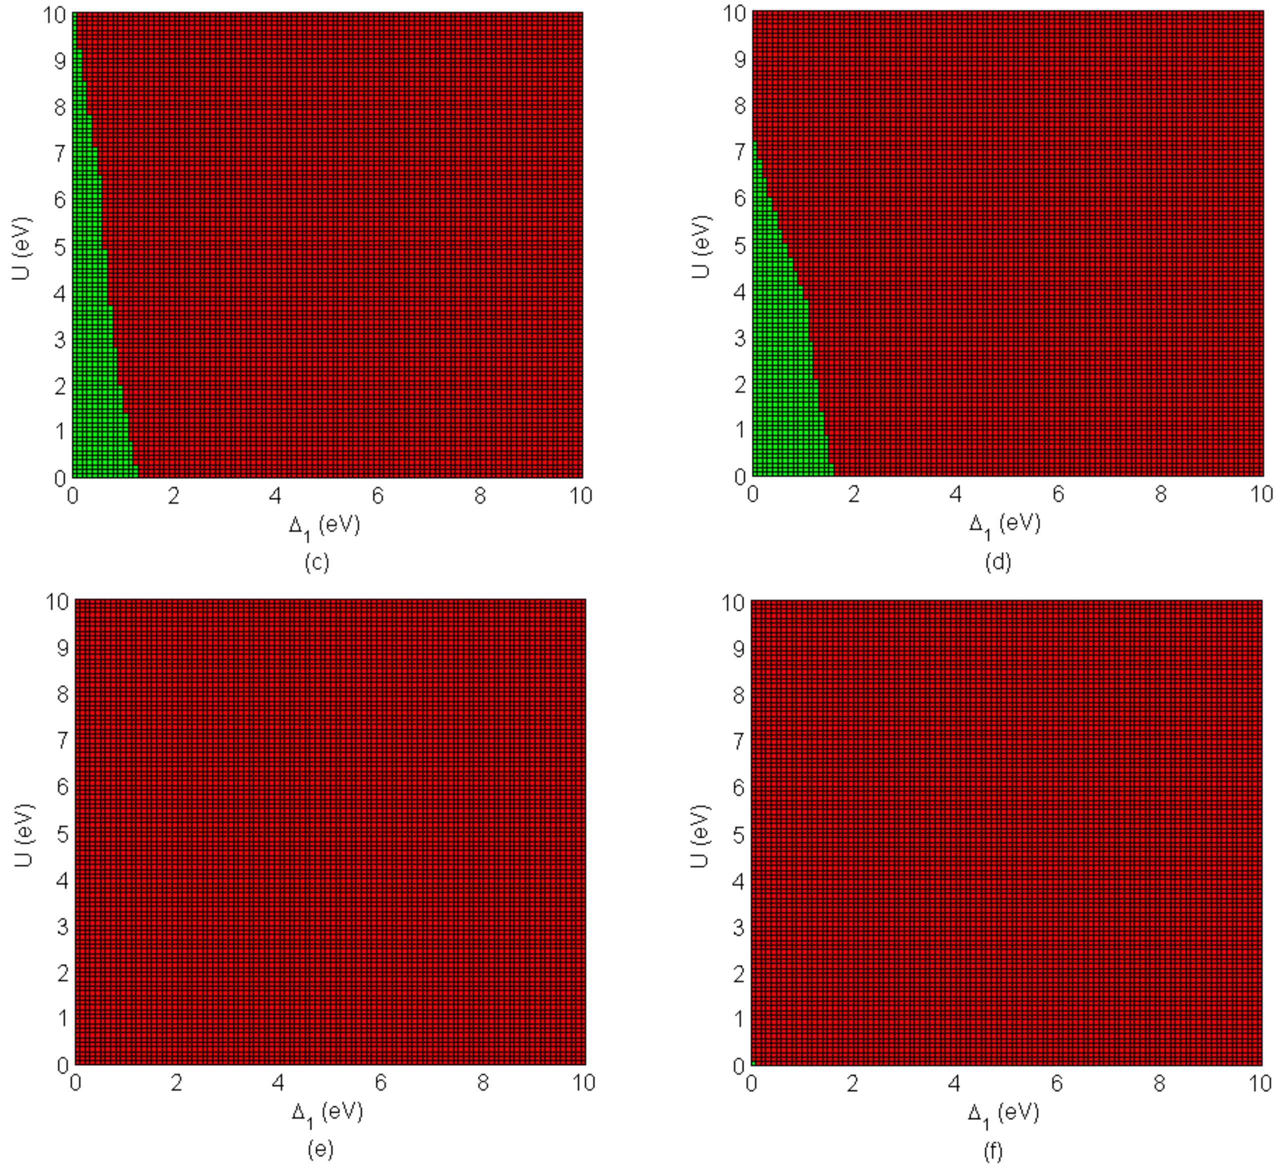


FIG. 2. Color maps of the parameter space $\Delta_1 \times U$ for rings with (a) $N = 3$ sites and $N_e = 3$ electrons with $\Delta_2 = 1, 2\, eV$, (b) $N = 5$ sites and $N_e = 5$ electrons with $\Delta_2 = 1\, eV$, (c) $N = 4$ sites and $N_e = 4$ electrons with $\Delta_2 = 0, 5\, eV$, (d) $N = 4$ sites and $N_e = 4$ electrons with $\Delta_2 = 1\, eV$, (e) $N_e$ even and not a multiple of four and (f) $N_e$ even and a multiple of four.

## IV. PERSISTENT CURRENT

### A. Persistent current in the Hubbard model

Figures on the left half of the page refer to the persistent current obtained through the Hubbard model (without the extra electronic interaction term $\hat{H}_I$) as a function of the magnetic flux $f = \phi/\phi_0$ that pierces the rings with (a) three sites and two electrons, (c) three sites and three electrons, (e) four sites and three electrons, (g) five sites and five electrons, (i) six sites and two electrons, and (k) six sites and six electrons. Note that, as pointed in the article, in the particular cases of Figs. 3(c) and (g), in which the rings have an odd number of sites and are at half-filling, the persistent current is $\phi_0/2$-periodic, instead of $\phi_0$-periodic.

Figures on the right half of the page refer to the same systems of the figures on the left, respectively, but now we show the persistent current as a function of the on-site repulsion, $U$. Notice that, as pointed out in the article, the absolute value of the persistent current always decreases with increasing $U$.

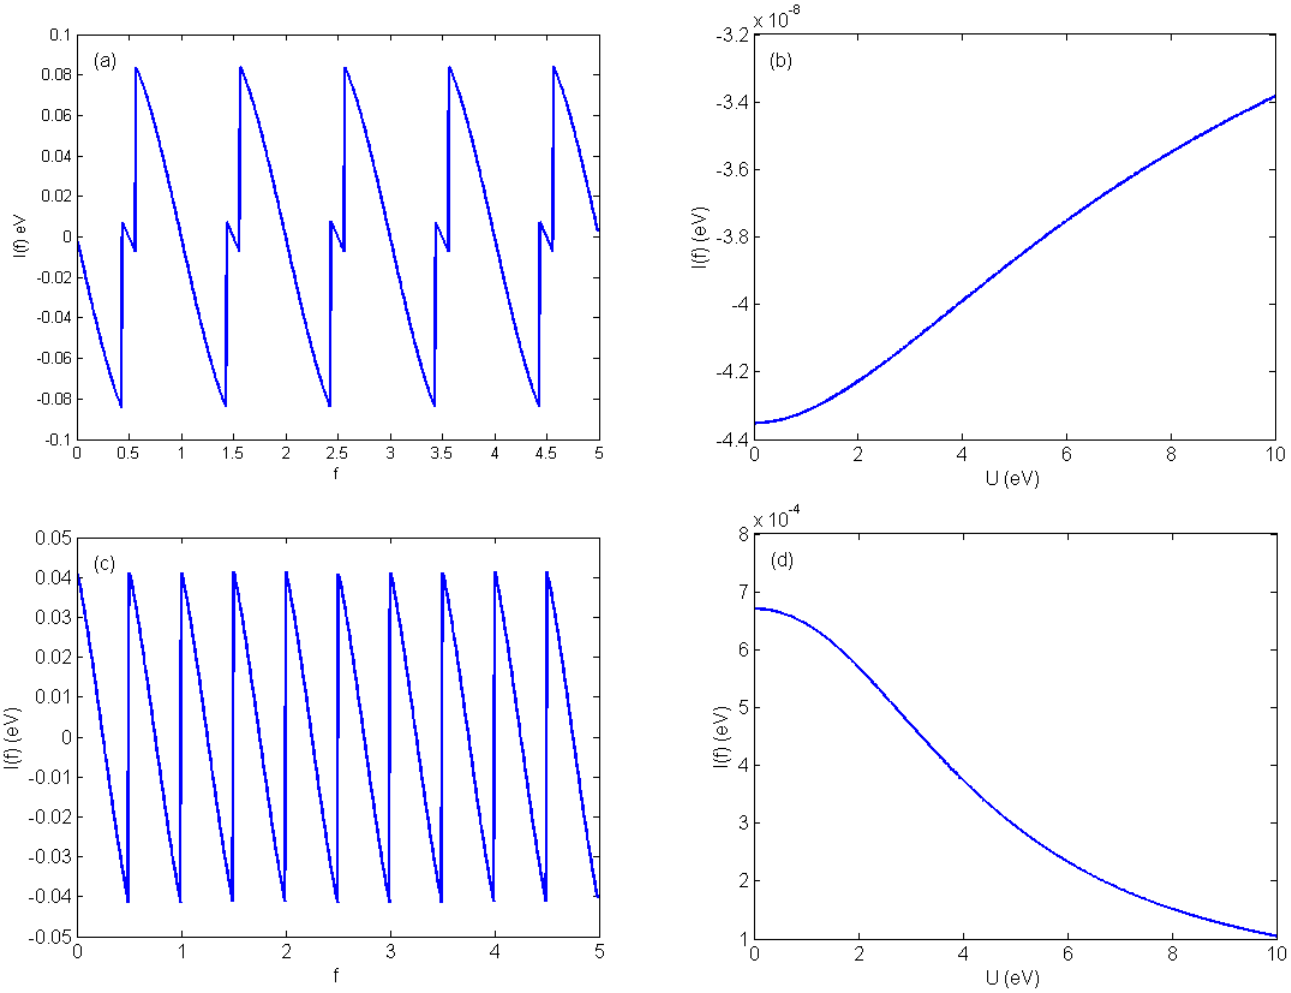

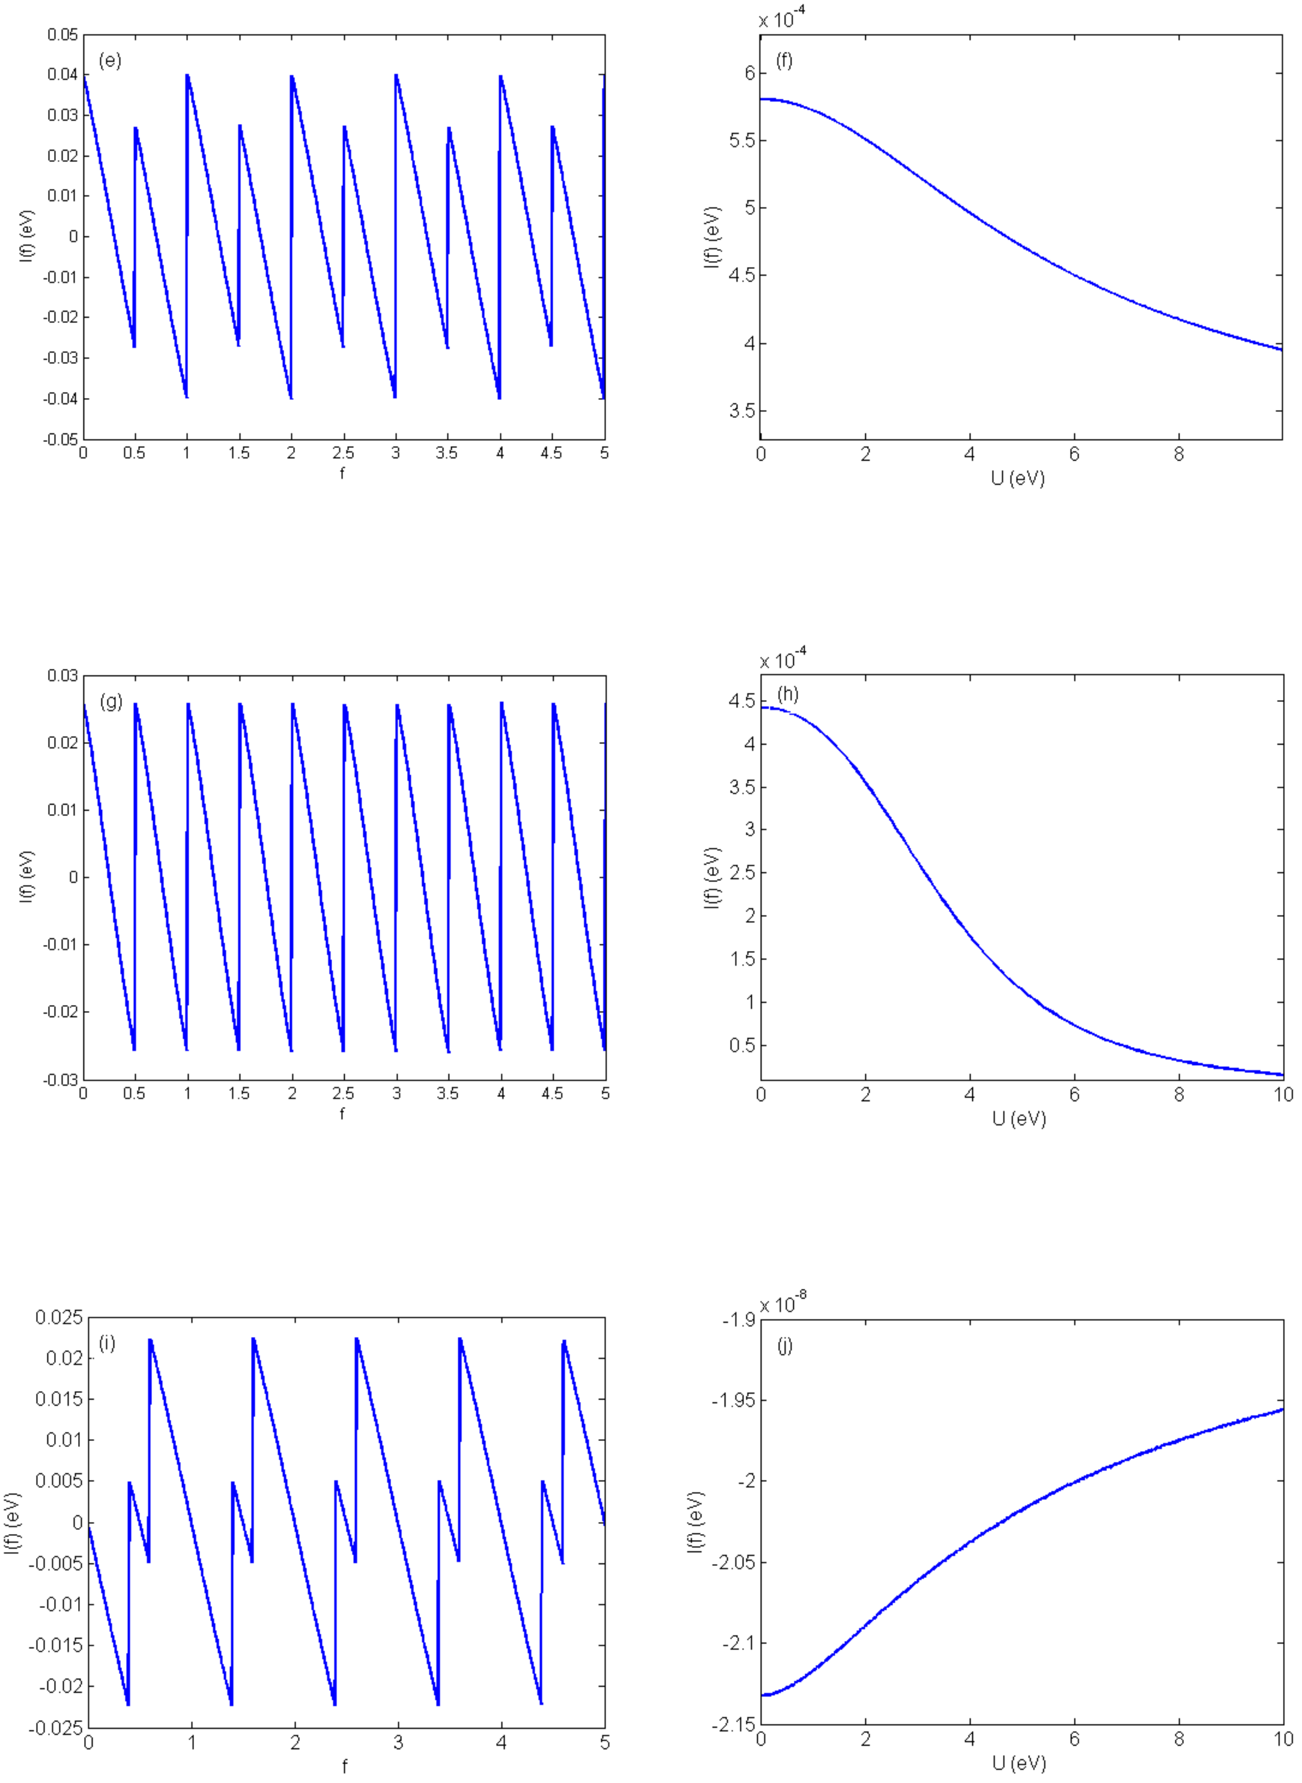
(e)
I(f) (eV)
f
(f)
x 10^-4
I(f) (eV)
U (eV)
(g)
I(f) (eV)
f
(h)
x 10^-4
I(f) (eV)
U (eV)
(i)
I(f) (eV)
f
(j)
x 10^-8
I(f) (eV)
U (eV)

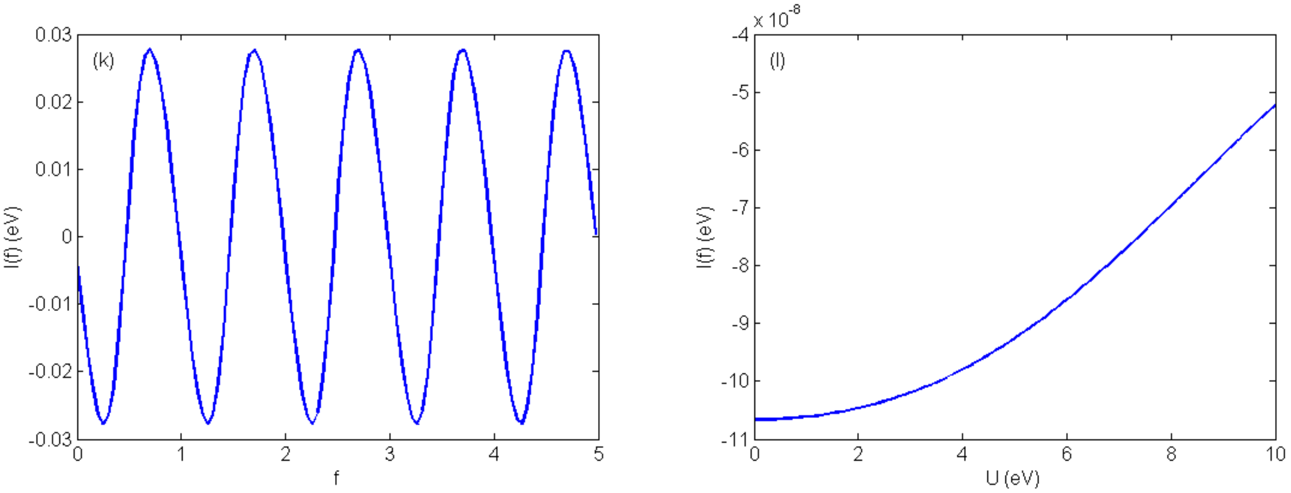


FIG. 3. Persistent current established in the ground state of rings with $N = 3$ sites and $N_e = 2$ electrons ((a) and (b)), $N = 3$ sites and $N_e = 3$ electrons ((c) and (d)), $N = 4$ sites and $N_e = 3$ electrons ((e) and (f)), $N = 5$ sites and $N_e = 5$ electrons ((g) and (h)), $N = 6$ sites and $N_e = 2$ electrons ((i) and (j)) and $N = 6$ sites and $N_e = 6$ electrons ((k) and (l)). In each of them we set the hopping parameter $t = 1eV$ and the lattice spacing $a = 1$Å, except in figures (i) and (j), where $a = 1,4$Å, and (k) and (l), in which $t = 2,5\,eV$ and $a = 1,4$Å. In figures (a), (c), (e), (g), (i) and (k), the persistent current is shown as a function of the magnetic flux that pierces the ring, with $U = 2\,eV$ fixed (except for the ring with six sites and six electrons, where we used $U = 10\,eV$). In figures (b), (d), (f), (h), (j) and (l), the persistent current is shown as a function of the on-site repulsion with $B = 2T$ fixed.

### B. Persistent current in our extension of the Hubbard model

Similarly to subsection IV A, figures on the left half of the page refer to the persistent current as a function of the magnetic flux that pierces the rings with (a) three sites and two electrons, (c) three sites and three electrons, (e) four sites and three electrons, (g) five sites and five electrons, (i) six sites and two electrons, and (k) six sites and six electrons. However, here the persistent currents are evaluated within our extension of the Hubbard model. In each figure on the left half page, there are two curves: the blue (solid) lines refer to a value of the on-site repulsion before the level crossing, *i.e.* for $U < U_0$ (see Fig. 1 in section I), whereas the green (dashed) lines refer to $U > U_0$. The insets in Figs. 4 show a zoom on the curves of the persistent current for small values of the magnetic flux $f$. Note that, indeed, $I(f)$ tends to a finite value as $f$ approaches zero only in the cases in which the number of electrons in the ring is odd.

Figures on the right half of the page show the persistent current as a function of the on-site repulsion parameter for the same systems of the left column, respectively. Again we have two curves: the blue (solid) lines refer to the Hubbard model (*i.e* $\Delta_1 = \Delta_2 = 0$), while the red (dashed) lines refer to $\Delta_1 \neq 0$ and/or $\Delta_2 \neq 0$. In order to ease the comparison between the persistent currents obtained with the Hubbard model and our extension thereof, both of them are normalized by $I_0$, the value of the persistent current in the absence of any electronic interaction (pure hopping model).

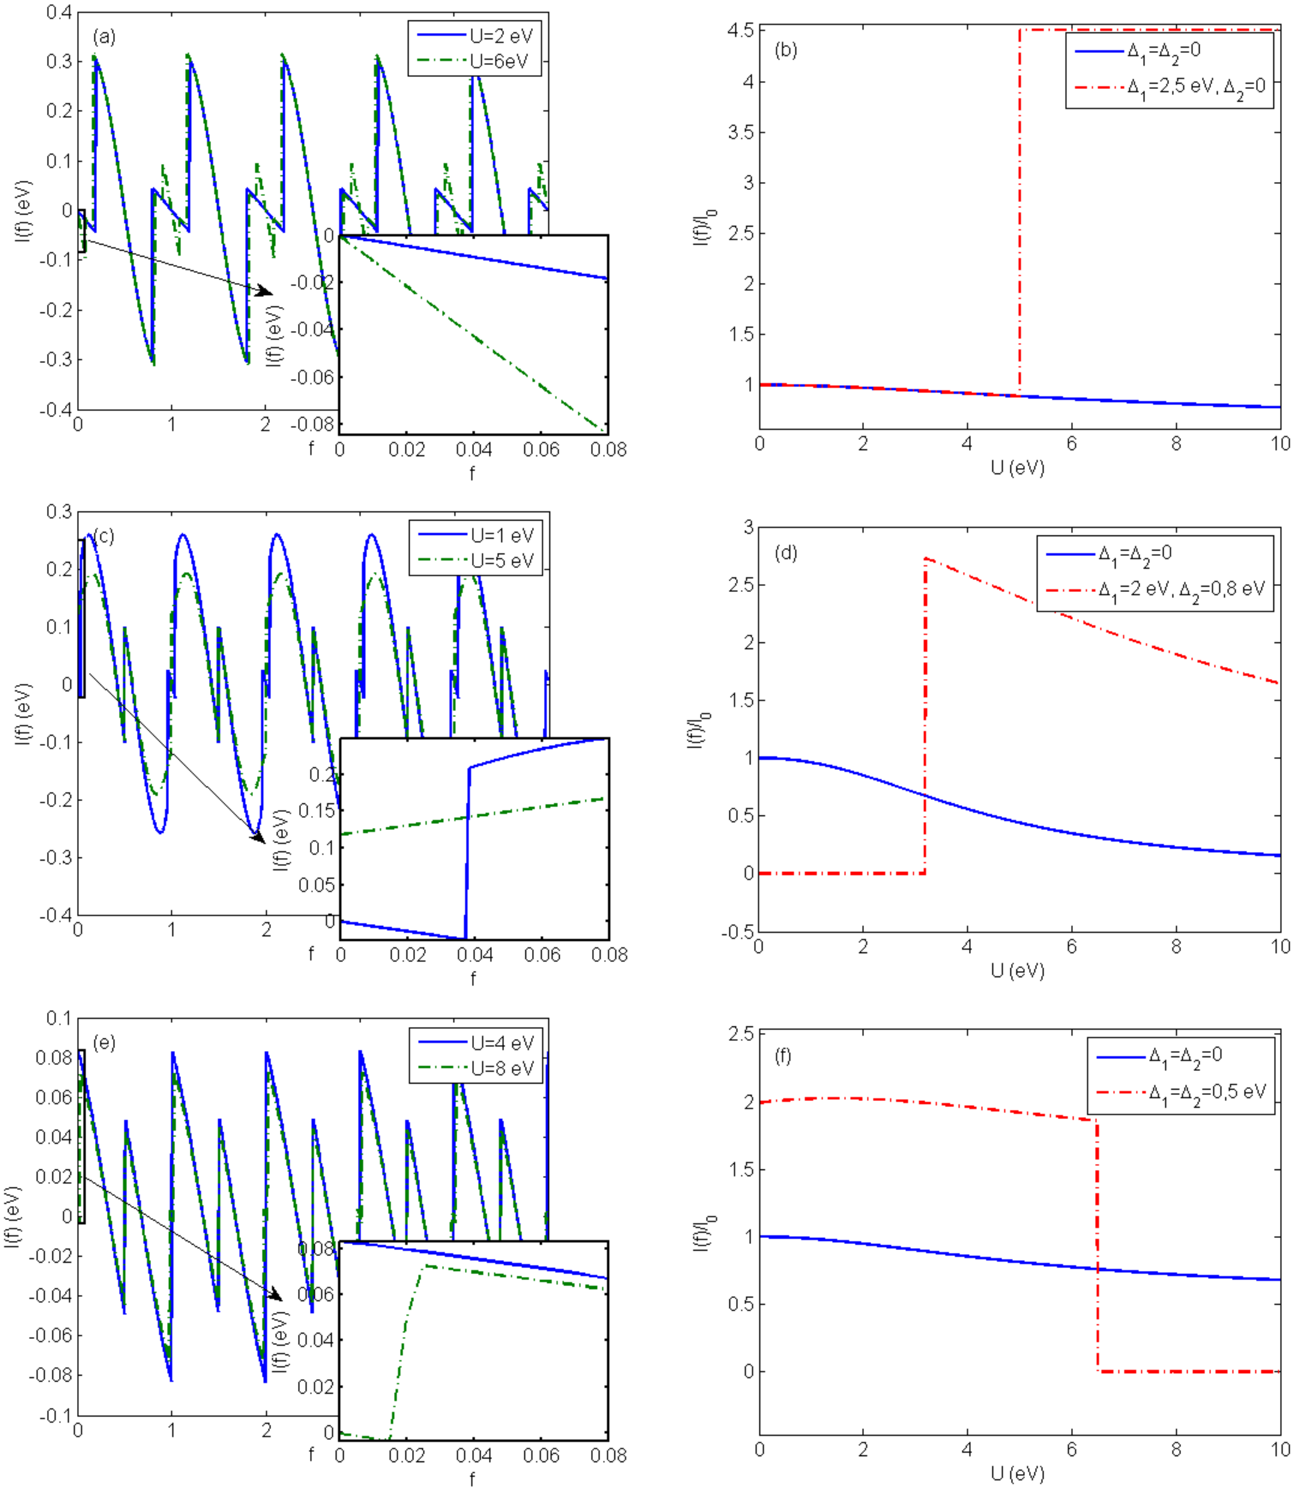
(a)
U=2 eV
U=6eV
I(f) (eV)
f
(b)
$\Delta_1=\Delta_2=0$
$\Delta_1$=2,5 eV, $\Delta_2$=0
$I(f)/I_0$
U (eV)
(c)
U=1 eV
U=5 eV
I(f) (eV)
f
(d)
$\Delta_1=\Delta_2=0$
$\Delta_1$=2 eV, $\Delta_2$=0,8 eV
$I(f)/I_0$
U (eV)
(e)
U=4 eV
U=8 eV
I(f) (eV)
f
(f)
$\Delta_1=\Delta_2=0$
$\Delta_1=\Delta_2$=0,5 eV
$I(f)/I_0$
U (eV)

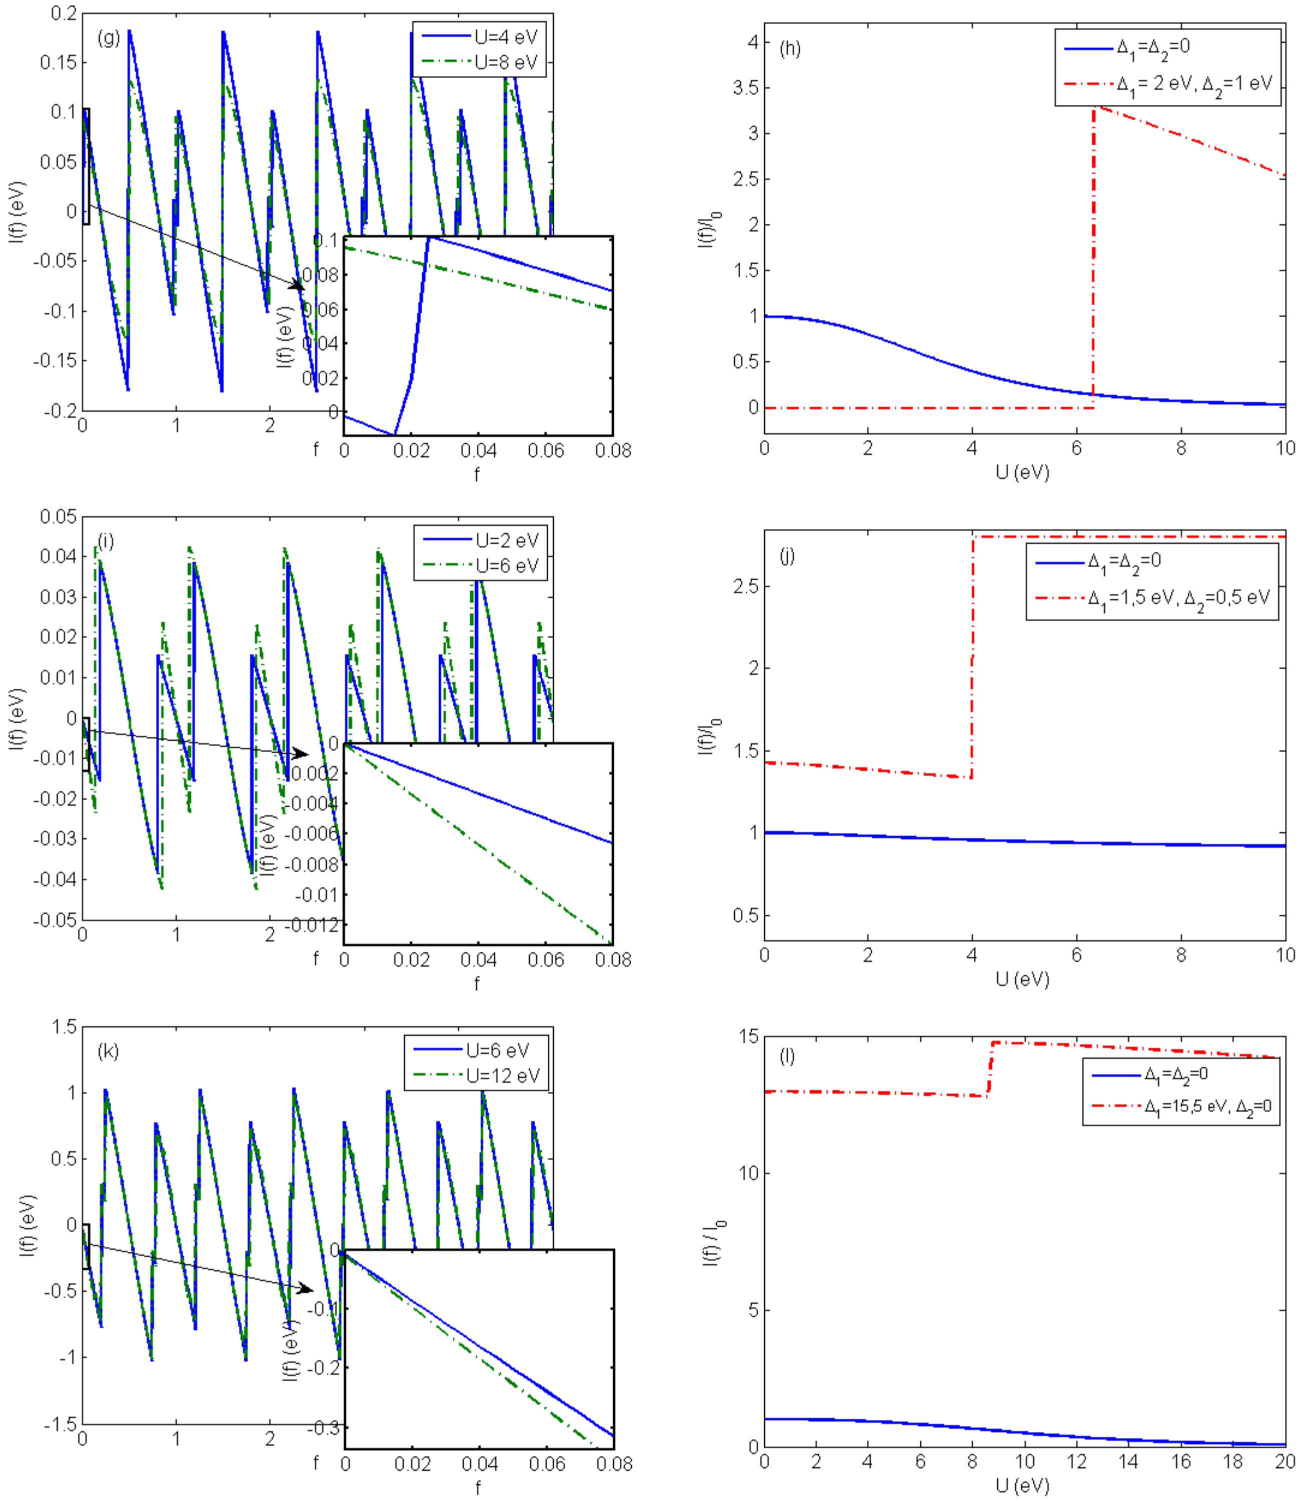


FIG. 4. Persistent current established in the ground state of rings with $N = 3$ sites and $N_e = 2$ electrons ((a) and (b)), $N = 3$ sites and $N_e = 3$ electrons ((c) and (d)), $N = 4$ sites and $N_e = 3$ electrons ((e) and (f)), $N = 5$ sites and $N_e = 5$ electrons ((g) and (h)), $N = 6$ sites and $N_e = 2$ electrons ((i) and (j)) and $N = 6$ sites and $N_e = 6$ electrons ((k) and (l)). In each of them we set the hopping parameter $t = 1eV$ and the lattice spacing $a = 1$Å, except in figures (i) and (j), in which $a = 1,4$Å, and (k) and (l), in which $t = 2,5\,eV$ and $a = 1,4$Å. In each of the figures (a), (c), (e), (g), (i) and (k), the persistent current is shown as a function of the magnetic flux that pierces the ring, with two distinct values of $U$ (indicated in the figures). The blue (solid) line refer to $U < U_0$, whereas the green (dashed) lines to $U > U_0$. The insets in these figures show a zoom in the curves of the persistent current for small values of $f$. The values of $(\Delta_1; \Delta_2)$ used in the figures on the left half of the page are: (a) $(2,5;0)\,eV$, (c) $(2;0,8)\,eV$, (e) $(0,5;0,5)\,eV$, (g) $(2;1)\,eV$, (i) $(1,5;0,5)\,eV$, and (k) $(15,5;0)\,eV$. In figures (b), (d), (f), (h), (j) and (l), the persistent current is shown as a function of the on-site repulsion with $B = 2T$ fixed and for two distinct sets of $(\Delta_1, \Delta_2)$ indicated in the figure. The blue (solid) lines refer to $\Delta_1 = \Delta_2 = 0$, whereas the green (dashed) lines to $\Delta_1 \neq 0$ or/and $\Delta_2 \neq 0$.

[1]H.; Göhmann F.; Klümper A.; Korepin V. E. Essler, F. H. L.; Frahm. *The One-Dimensional Hubbard Model*. United Kingdom: Cambridge University Press, 2005.

[2]Wei Bo-Bo; Gu Shi-Jian; Lin Hai-Qing. Persistent currents in the one-dimensional mesoscopic hubbard ring. *J. Phys.: Condens. Matter*, 20:1, 2008.
